# Supplementary material for: Comment on "Unconventional Fermi Surface Instabilities in the Kagome Hubbard Model" by M. Kiesel, C. Platt, and R. Thomale, Phys. Rev. Lett. {\bf 110}, 126405 (2013)
Source: arXiv:1809.03931 source file (2018-09-14)
Supplement: Supplementary file 1 [file SM_kagome.pdf]

# Supplemental Materials for the Comment on "Unconventional Fermi Surface Instabilities in the Kagome Hubbard Model" by M. Kiesel, C. Platt, and R. Thomale, Phys. Rev. Lett. 110, 126405 (2013)

Li-Han Chen,[1] Zhen Liu,[1] and Jian-Ting Zheng[1,2,*]

[1]*National Laboratory of Solid State Microstructures & School of Physics, Nanjing University, Nanjing, 210093, China*
[2]*Collaborative Innovation Center of Advanced Microstructures, Nanjing University, Nanjing 210093, China*

Here we describe the technical details involved to obtain the results in the main text of the comment.

## S1. HAMILTONIAN

The Hamiltonian of the kagome-Hubbard model is, in real space,

$$H = -t \sum_{\langle ij\rangle\sigma} (c_{i\sigma}^\dagger c_{j\sigma} + \text{h.c.}) + U \sum_i n_{i\uparrow} n_{i\downarrow} - \mu \sum_i n_i \quad \text{(S1)}$$

Here $\langle ij\rangle$ denotes a nearest-neighbor (NN) bond (to be counted only once), $c_{i\sigma}$ is the electron annihilation operator at site $i$ and of spin $\sigma = \uparrow / \downarrow$, $n_{i\sigma} = c_{i\sigma}^\dagger c_{i\sigma}$, $n_i = n_{i\uparrow} + n_{i\downarrow}$, $U$ is the local Hubbard interaction, and finally $\mu$ is the chemical potential. Notice that there are three sublattices in the kagome lattice, or in other words, three unequivalent sites within a primitive unitcell. See Fig.S1(a)-(c) for illustration. On the other hand, $\mu = 0$ corresponds to, in the free limit, the van Hove level discussed in Refs.1–3, with electron density $n_e = 5/6$ (per site). In Ref.1 the interactions on NN bonds and electron density away from 5/6 are also considered. Here we are only interested in the van Hove level, since the system is most susceptible to instabilities when interactions are switched on. We consider local-interaction only, since this case is easiest to check.

## S2. HATREE-FOCK AND DYNAMICAL MEAN FIELD CALCULATIONS

We first consider local ordering of spin moment, either in the form of uniform ferromagnetism (FM), or in the form of the 120° antiferromagnetic (AFM) alignment of the spin moment (periodic from unitcell to unitcell), see Fig.S1(a) and (b). Both of these orders have zero crystal momentum, and can be handled simultaneously by calculating the bare spin susceptibility at zero frequency and zero momentum, which is a matrix in the sublattice basis, with the elements

$$D_0^{ab} = -\frac{T}{N} \lim_{\mathbf{q}\to 0} \sum_{\mathbf{k}\omega_n} G_{\mathbf{k}}^{ab}(i\omega_n) G_{\mathbf{k}+\mathbf{q}}^{ba}(i\omega_n), \quad \text{(S2)}$$

where $a$ and $b$ refer to sublattice, $T$ is the temperature, $N$ the number of unitcells, and $G_{\mathbf{k}}(i\omega_n)$ is the single-particle Green's function at momentum $\mathbf{k}$ and Matsubara

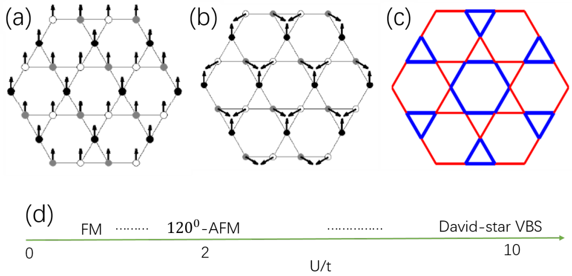


FIG. S1: Illustration of (a) FM, (b) 120°-AFM, and (c) David-star VBS orders on the kagome lattice. The arrows in (a) and (b) indicate the direction of the spin moment. In the variational Hamiltonian, these arrows can also be taken as the variational field $\mathbf{h}_i$, with amplitude $h_{\rm FM}$ in (a) and $h_{120^\circ-\rm AFM}$ in (b). The blue bonds in (c) form hexgons and triangles. In the variational Hamiltonian, the blue/red bonds are associated with $\pm\Delta t_{\rm David-star}$, and the onsite energy is shifted by $V_i = \pm V_{\rm cdw}$ on the blue hexagons/triangles. (d) A schematic phase diagram along the $U$-axis of the kagome-Hubbard model from our numerical results. The dots indicate possible transition between neighboring phases.

frequency $\omega_n = (2n+1)\pi T$. Explicitly,

$$G_{\mathbf{k}}^{ab}(i\omega_n) = \sum_\alpha \frac{\langle a|\mathbf{k}\alpha\rangle\langle\mathbf{k}\alpha|b\rangle}{i\omega_n - \epsilon_{\mathbf{k}\alpha}}, \quad \text{(S3)}$$

where $\alpha$ indicates a single-particle state $|\mathbf{k}\alpha\rangle$, with eigen energy $\epsilon_{\mathbf{k}\alpha}$, of the free part of the Hamiltonian. After completing the summation over Matsubara frequencies, we are left with

$$D_0^{ab} = \frac{1}{N} \sum_{\mathbf{k}\alpha\beta} \langle a|\mathbf{k}\alpha\rangle\langle\mathbf{k}\alpha|b\rangle\langle b|\mathbf{k}\beta\rangle\langle\mathbf{k}\beta|a\rangle \times \lim_{\mathbf{q}\to 0} \frac{f(\epsilon_{\mathbf{k}\alpha}) - f(\epsilon_{\mathbf{k}+\mathbf{q},\beta})}{\epsilon_{\mathbf{k}+\mathbf{q},\beta} - \epsilon_{\mathbf{k}\alpha}}, \quad \text{(S4)}$$

where $f(\epsilon) = 1/(e^{\epsilon/T}+1)$ is the Fermi function. *The so-called matrix-element interference, emphasized in Ref.1–3, is reflected here by the coherence factors in the first line of the above equation.* The renormalized susceptibility is, in the random phase approximation (RPA), and in matrix form,

$$D = \frac{D_0}{1 - UD_0}, \quad \text{(S5)}$$

where we used the fact that the Hubbard $U$ is diagonal in the sublattice basis. Note the identity matrix is written as 1 in the denominator. The Stoner instability is signaled by the divergence of $D$. This occurs if the eigenvalue $\chi$ of $D_0$ meets $1 = U\chi$. According to our calculations, the $3 \times 3$ hermitian matrix $D_0$ has three eigenvalues, one nondegenerate and the other two degenerate. The former is associated with the eigenvector $(1,1,1)^t/\sqrt{3}$, corresponding to uniform FM order within the unitcell, see Fig.S1(a). The latter ones are associated with the eigenvectors $(1,-1,0)^t/\sqrt{2}$ and $(1,1,-2)^t/\sqrt{6}$. Hatree-Fock mean field theory (HFMFT) calculation shows that they recombine to form the non-colinear 120°-AFM, see Fig.S1(b). The Stoner instability lines are plot in Fig.1(a) of the main text. We need to emphasize that the phase boundary is determined by the first Stoner instability as the temperature is decreased from high to low. This determines the ordered phase at low $T$, which is exactly identical to that from HFMFT. In the main text, we show that FM is absent for $U > U_0 \sim 1.57t$, yielding to 120°-AFM. Note that both forms of spin orders are over-emphasized by RPA/HFMFT. So if FM is not the order in RPA or HKMFT, it is unlikely that longer-range fluctuations (in space and imaginary time) beyond HFMFT could rescue FM again.

To check the reliability of the RPA/HFMFT, we go one step further by resorting to dynamical mean field theory (DMFT).[4] The DMFT solves a single quantum impurity enbedded in a dynamical environment, exactly and self-consistently, and is known to be much better than HFMFT since local quantum fluctuations are taken into account. We solve the quantum impurity problem using the numerical renormalization group (NRG).[5] For the uniform FM phase, we take one site as the impurity, and the rest the environment. For the 120°-AFM, the spin order is non-colinear. We need to take care of three unequivalent spin moments. However, assuming the self-energy is local, we verified that the self-energy matrix (in spin basis) on one site can be rotated to that on the other site by ±120° SU(2) rotations. Therefore, it is still possible to take one site as the quantum impurity (for which we take the spin-diagonal basis), and the rest as the environment, with the above necessary rotations in mind to form the lattice Green's function, or in the Hilbert transformation to get the hybridization kernel. A similar but simpler case is the AFM on square lattice, where there are two unequivalent spin sites. The subsequent calculations are standard. We start from a self-energy capable of inducing the respective form of spin order, and iterate until the hybridization kernel or the self-energy converges. The chemical potential is tuned concurrently to fix the local charge density at 5/6. Our DMFT results (for discrete values of $U$) in Fig.1(b) show FM can not survive at $U \geq 2t$, where 120°-AFM is stable. This is consistent with RPA/HFMFT qualitatively. But quantitatively, the size of the moment is reduced by local quantum fluctuations captured by DMFT. For example, at large $U$, the spin moment $M \to 1/2$ in HFMFT, but $M < 1/4$ in DMFT and begins to drop for $U > 8t$. The local density of states at $U = 10t$ in the inset of Fig.1(b) shows the opening of a Mott gap. We then switch to a strong coupling theory below.

## S3. VARIATIOAL QUANTUM MONTE CARLO IN THE LARGE-$U$ LIMIT

The MFT's discussed above are limited to local spin orders. At large $U$, the Mottness comes into play, and a better account of spin-spin correlation and renormalization of kinetic energy at the Hamiltonian level is captured by the $t$-$J$ model,

$$\begin{aligned} H_{t-J} = & -t\sum_{\langle ij\rangle\sigma}(Pc_{i\sigma}^\dagger c_{j\sigma}P + \text{h.c.}) \\ & +J\sum_{\langle ij\rangle}(\mathbf{S}_i\cdot\mathbf{S}_j - n_i n_j/4), \end{aligned} \quad \text{(S6)}$$

where $P = \Pi_i(1 - n_{i\uparrow}n_{i\downarrow})$ projects away double occupancy, $J = 4t^2/U$, and $\mathbf{S}_i$ is the electron spin. We drop the chemical potential term, since we are going to work in the canonical ensemble. This model is much easier to perform variational quantum Monte Carlo (VQMC) than the Hubbard model, since the Mott physics is already built in. In the following we consider $U = 10t$ so that $J = 0.4t$.

We consider the following variational Hamiltonian,

$$\begin{aligned} H_v = & -\sum_{\langle ij\rangle\sigma}(t + \Delta t_{\langle ij\rangle})(c_{i\sigma}^\dagger c_{j\sigma} + \text{h.c.}) \\ & -\sum_{i\sigma\sigma'} c_{i\sigma}^\dagger \mathbf{h}_i\cdot\vec{\sigma}_{\sigma\sigma'}c_{i\sigma'} + \sum_i n_i V_i \\ \to & \sum_{i\sigma,j\sigma'} c_{i\sigma}^\dagger h_{i\sigma,j\sigma'}c_{j\sigma'}. \end{aligned} \quad \text{(S7)}$$

Here $\{\mathbf{h}, \Delta t, V\}$ are variational parameters. The single-particle states of $H_v$ is given by

$$\sum_{j\sigma'} h_{i\sigma,j\sigma'}\phi_n(j\sigma') = \epsilon_n\phi_n(i\sigma), \quad \text{(S8)}$$

where $\epsilon_n$ is the $n$-th eigenvalue, and we prescribe

$$\epsilon_1 \leq \epsilon_2 \leq \epsilon_3 \cdots . \quad \text{(S9)}$$

The ground state of $H_v$ is

$$|v\rangle = \Pi_{n\leq N_e}\left(\sum_{i\sigma}\phi_n(i\sigma)c_{i\sigma}^\dagger\right)|0\rangle = \sum_R D_R|R\rangle, \quad \text{(S10)}$$

where $N_e$ is the total number of electrons, $|0\rangle$ is the vacuum, $|R\rangle$ is a real-space configuration state of the electrons with a Slater-determinant coefficient $D_R$. The physical energy is

$$E = \frac{\langle v|PH_{t-J}P|v\rangle}{\langle v|P|v\rangle}, \quad \text{(S11)}$$

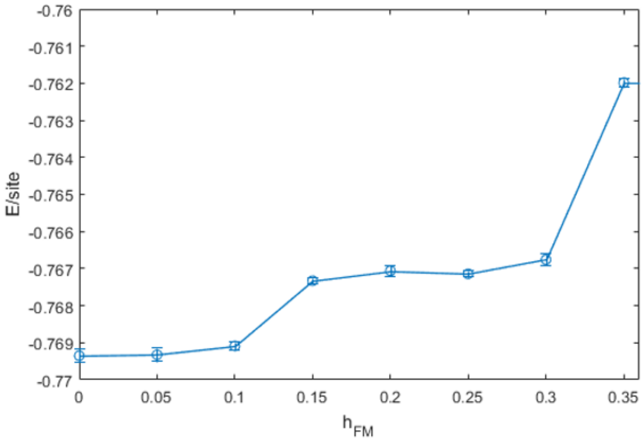


FIG. S2: Energy (per site) versus $h_{\rm FM}$ for the FM phase.

and is calculated by standard VQMC. If necessary, we optimize all independent variational parameters in $\{\mathbf{h}, \Delta t, V\}$ automatically using the method detailed in Ref.6. We update the configurations on sites and on bonds, and define the scanning of the entire lattice as a MC step. We use 32000 steps for thermalization and 128000 steps (samples) for statistical average. The acceptance ratio is typically $0.27 \sim 0.3$ during attempts to update the configuration states. The states at two successive MC steps are essentially statistically independent. This is seen by the fact that reducing the sampling frequency does not lead to any change of the results within statistical error.

We consider six primitive unicells along each of the two principle axes of the kagome lattice, so the total number of sites is $6 \times 6 \times 3$. The result is insensitive to the boundary conditions for the fermion states but we set them antisymmetric for definiteness. We insert $N_e = 90$ electrons in total, so that the average filling is 5/6 per site.

We now consider the FM order. This is handled by setting $\mathbf{h}_i$ in the configuration of Fig.S1(a), with the magnitude $h_{\rm FM}$. On the other hand we set $\Delta t_{\langle ij\rangle} = 0$ and $V_i = 0$. A finite $h_{\rm FM}$ can induce uniform FM moment along $y$. Note that $\mathbf{h}_i$ in this form mixes spin-up and spin-down. The advantage is we are able to tune the FM moment continuously, plus enhanced self-averaging. The disadvantage is we need to deal with a twice-larger dimension of the Slater determinant in MC, as compared to the spin-diagonal case, limiting the lattice size we can reach. Fig.S2 shows the energy increases monotonically as $h_{\rm FM}$ increases, ruling out the possibility of FM order.

Next we consider the 120°-AFM and David-star VBS, see Fig.S1(b) and (c). These orders may compete, so we treat them simultaneously. Note that in the David-star pattern, there are enhanced bonds on hexagons and triangles. For best optimization, we also include a charge potential to tune the chage density imbalance on them. These considerations lead us to set $\mathbf{h}_i$ in the configuration of Fig.S1(b), with the magnitude $h_{120^\circ-{\rm AFM}}$, and set in the David-star pattern $\Delta t_{\langle ij\rangle} = \pm\Delta t_{\rm David-star}$ for enhanced/weaked bonds and $V_i = \pm V_{\rm cdw}$ for sites on the enhanced hexagons/triangles, see Fig.S1(c). The variational process is vividly shown in Fig.1(c) in the main text, as trajectories in the energy landscape. The small wiggling of the trajectories follows from statistical errors. The result shows that the David-star VBS survives, while the other parameters, $h_{120^\circ{\rm AFM}}$ and $V_{\rm cdw}$, vanish as the energy is optimized to the minimum.

In retrospection, our VQMC results are not even new. Systematic results near half filling of the kagome model are known in the literature.[7–9] Our new input is the spin order (in various forms), which turns out to be irrelevant indeed. Therefore, our results confirm those in Ref.7–9, where the lattice size is relatively larger (up to $8 \times 8 \times 3$). In combination, the finite-size effect is negligible for our purpose.

## S4. SUMMARY

To summarize, in the kagome-Hubbard model at the van Hove singularity, FM is possible for small $U$, then 120°-AFM enters at least for $U > 2t$, and for even larger $U$, the system is in the David-star VBS state. A schematic phase diagram is drawn in Fig.S1(d). We should mention that the FM and AFM states are defined either at zero temperature or in the mean field sense at finite temperatures, since a continuous symmetry can not be broken at finite temperature by Mermin-Wagner theorem. The VBS is rather different. It only breaks discrete symmetry, and hence can order in two-dimension even at finite temperatures. In fact the VBS state generates a full gap for quasiparticle excitations, and should be much more stable than the other states, once established.

The fact that FM is absent at large $U$ in MFT acts strongly against its persistence in Ref.1, since MFT should have over-emphasized any orders within its scope. Therefore, Ref.1 may have biased FM more than MFT does, in such a way that the 120°-AFM and David-star VBS at larger $U$ are unfortunately overlooked.

* Electronic address: mf1722040@smail.nju.edu.cn

1 M. Kiesel, C. Platt, and R. Thomale, Phys. Rev. Lett. **110**, 126405 (2013).
2 S. L. Yu and J. X. Li, Phys. Rev. B **85**, 144402 (2012).
3 W. S. Wang, Z. Z. Li, Y. Y. Xiang, and Q. H. Wang, Phys. Rev. B **87**, 115135 (2013).
4 A. Georges, G. Kotliar, and W. Krauth, Rev. Mod. Phys. **68**, 13-125 (1996).

[5] R. Bulla, T. A. Costi, T. Pruschke, Rev. Mod. Phys. **80**, 395 (2008).

[6] J. Toulouse and C. J. Umrigar, J. Chem. Phys. **126**, 084102 (2007).

[7] S. Guertler and H. Monien, Phys. Rev. B **84**, 174409 (2011).

[8] S. Guertler and H. Monien, Phys. Rev. Lett. **111**, 097204 (2013).

[9] S. Guertler, Phys. Rev. B **90**, 081105 (2014).
